# Supplementary material for: Learning shape resonances from the stabilization method
Source: arXiv:2605.28437 source file (2026-10-07)
Supplement: Supplementary file 1 [file supplement.tex]

\documentclass[prb,twocolumn]{revtex4-1} 
% The line above defines the type of LaTeX document.
% Note that AJP uses the same style as Phys. Rev. B (prb).

% The % character begins a comment, which continues to the end of the line.

\usepackage{amsmath}  % needed for \tfrac, \bmatrix, etc.
\usepackage{amsfonts} % needed for bold Greek, Fraktur, and blackboard bold
\usepackage{graphicx} % needed for figures

%%%%%%%%%%%%%%%%% CUSTOM PACKAGES AND COMMANDS %%%%%%%%%%%%%%%%%%%%%

\usepackage[group-digits = false]{siunitx}
\usepackage{verbatim}
\usepackage{physics}
\usepackage[version=4]{mhchem}

\usepackage{amssymb}
\usepackage{mathtools}
\usepackage{bbold}

\usepackage{booktabs}
\usepackage{tabularx}
\usepackage{float}

\usepackage[caption=false]{subfig}

\usepackage{tikz}
\usetikzlibrary{patterns}
\usetikzlibrary{arrows.meta}

\usepackage{ifthen}

\usepackage{hyperref}
\hypersetup{colorlinks=true, citecolor=blue, urlcolor=blue, linkcolor=blue}
\usepackage{cleveref}

%%%%%%%%%%%%%%%%%%%%%%%%%%%%%%%%%%%%%%%%%%%%%%%%%%%%%%%%%%%%%%%%%%%%

\setcounter{equation}{0}
\setcounter{figure}{0}
\setcounter{table}{0}

\begin{document}

% Be sure to use the \title, \author, \affiliation, and \abstract macros
% to format your title page.  Don't use lower-level macros to  manually
% adjust the fonts and centering.

\title{Supplementary Material\\for ``Learning shape resonances from the stabilization method''}

\author{Daniel Kromm}
\email{daniel.kromm@tu-darmstadt.de}
\affiliation{Technische Universität Darmstadt, Department of Physics, Institut f\"ur Kernphysik, 64289 Darmstadt, Germany}
\author{Hans-Werner Hammer}
\email{Hans-Werner.Hammer@physik.tu-darmstadt.de}
\affiliation{Technische Universität Darmstadt, Department of Physics, Institut f\"ur Kernphysik, 64289 Darmstadt, Germany}
\affiliation{ExtreMe Matter Institute EMMI and Helmholtz Forschungsakademie Hessen für FAIR (HFHF),
GSI Helmholtzzentrum f{\"u}r Schwerionenforschung GmbH, 64291 Darmstadt, Germany}
\author{Artem Volosniev}
\email{artem@phys.au.dk}
\affiliation{Department of Physics and Astronomy, Aarhus University, Aarhus,
DK-8000, Denmark}
\affiliation{ExtreMe Matter Institute EMMI,
GSI Helmholtzzentrum f{\"u}r Schwerionenforschung GmbH}

% See the REVTeX documentation for more examples of author and affiliation lists.

\date{\today}

% AJP requires an abstract for all regular article submissions.
% Abstracts are optional for submissions to the "Notes and Discussions" section.

\maketitle

\section{Dependence on Method Parameters and Fit Interval}
\label{app:robustness}
All three methods introduced in the main text involve auxiliary choices that are not fixed by the underlying data, such as the selection of eigenstates, averaging ranges, or fit intervals. While these choices do not affect the formal definition of the methods, they can influence the numerical extraction of resonance parameters in practice.

In this supplementary material, we analyze the sensitivity of the extracted resonance energy and width with respect to these method-specific parameters. This serves both to quantify the robustness of each approach and to justify the parameter choices used in the main text.

For simplicity and clarity, we restrict the analysis to the lowest resonance of the repulsive delta-shell potential with coupling $G=20$. This case provides a well-defined and narrow resonance, allowing for a controlled comparison of parameter dependencies across the different methods.

\subsection{Fit to Energy Levels}
The direct fit to an energy level requires the selection of a specific eigenstate $N$. Since the appearance of a plateau changes with increasing $N$, it is important to assess the dependence of the extracted resonance parameters on this choice.

To this end, we performed the analysis for $N=5,10,15$. The resulting resonance parameters, together with the exact values, are listed in Table~\ref{tab:fit_N_analysis}. We find that the extracted resonance energy is largely insensitive to the choice of $N$. In contrast, the width is systematically overestimated, with the deviation increasing for larger $N$. This suggests that one should avoid choosing $N$ too large. On the other hand, very small values of $N$ should also be avoided, as the corresponding plateau lies too close to the interior region, where finite-volume effects are more pronounced. Based on this trade-off, we choose $N=5$ for the extraction of resonance parameters in the main text.

\begin{table}[t]
    \caption{Values of lowest resonance for $G=20$ extracted from a direct fit to different energy levels $E_N(L)$. Energies and widths are given in units of $\hbar^2/(2ma^2)$.}
    \label{tab:fit_N_analysis}

    \begin{ruledtabular}
    \begin{tabular}{c c c}
        $N$ & $E_\mathrm{r}$ & $\Gamma$ \\
        \hline
        exact & $8.97$ & $0.246$ \\
        $5$   & $8.97$ & $0.258$ \\
        $10$  & $8.97$ & $0.271$ \\
        $15$  & $8.97$ & $0.284$ \\
    \end{tabular}
    \end{ruledtabular}
\end{table}

A second source of systematic uncertainty arises from the choice of the fit interval. We define the fit region as a symmetric interval around the center of the plateau. The plateau boundaries are identified using the second derivative $E_N''(L)$, which exhibits a local maximum and minimum around the stabilized region (see Fig.~\ref{fig:plateau_boundaries}). These extrema define the edges of the plateau.

\begin{figure}[t]
    \centering
    \includegraphics[width=1\linewidth]{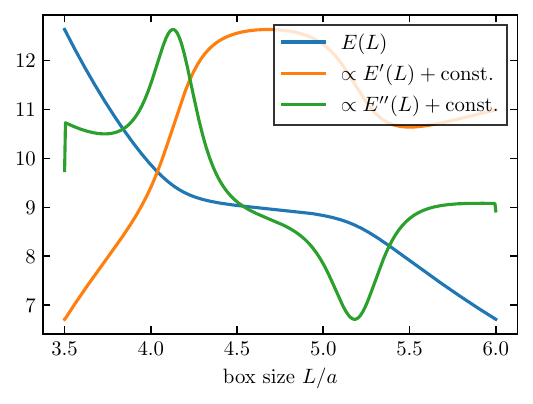}
    \caption{Energy level $N=5$ for $G=20$ displaying the plateau corresponding to the lowest  resonance. For identification of the plateau the first two derivatives are plotted (shifted and rescaled to fit in the range of the energy line).}
    \label{fig:plateau_boundaries}
\end{figure}

To quantify the dependence on the fit interval, we vary its length between $10\%$ and $50\%$ of the full plateau width (see Fig.~\ref{fig:fit_analysis}). We observe that the extracted resonance energy shows only a very weak dependence on the chosen interval. The width exhibits a somewhat stronger, but still moderate, dependence. In both cases, the variation decreases as the fit interval is reduced.

\begin{figure*}[t]
    \centering
    \includegraphics[width=1\linewidth]{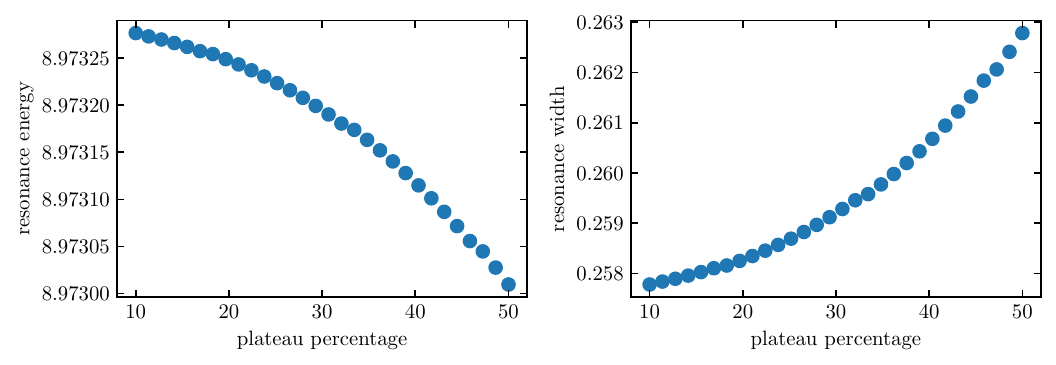}
    \caption{Resonance parameters from direct fit of $N=5$ state for $G=20$ for different fit interval length. This length is given in units the plateau length.}
    \label{fig:fit_analysis}
\end{figure*}

In our main analysis, we therefore choose a relatively small fit interval corresponding to $20\%$ of the plateau width. This choice represents a compromise: it is sufficiently small to minimize systematic variations, while still large enough to ensure a stable and reliable fit.

\subsection{Fit to Density of States}
For the DOS-based method, several auxiliary choices enter the analysis. In addition to the selection of a representative eigenstate and the fit interval, one must also specify how many neighboring states are included in the averaging procedure used to construct the DOS.

We begin by investigating the dependence on the choice of the central state. Averaging over three consecutive plateaus, we extract resonance parameters for $N=5,10,15$, where in each case the DOS is constructed from the states $N,N-1,N-2$. The resulting energies and widths agree within three significant digits. This indicates that the method is largely insensitive to the specific choice of the plateau, and we therefore fix $N=10$ in the main analysis.

Next, we vary the number of states included in the averaging procedure. Comparing averages over one, three, and five consecutive plateaus, we again find that both energies and widths agree within three significant digits. This demonstrates that the DOS construction is highly stable with respect to this parameter. In the main analysis, we choose to average over three plateaus as a reasonable compromise between smoothness and locality.

Finally, we consider the choice of the fit interval. In contrast to the direct-fit method, the DOS is already a smooth function of energy, and the fit interval is defined directly in energy space. For the main analysis, we choose a symmetric interval around the Lorentzian peak. To determine its extent, we proceed as follows. On each side of the peak, we determine two characteristic distances: (i) the distance from the peak to the nearest local minimum, and (ii) twice the distance from the peak to the point where the DOS reaches half of its maximum value. This yields four candidate distances in total (two per side). From these, we select the smallest distance and define a symmetric fit interval of total length equaling twice this distance centered at the peak.

To assess the sensitivity to this choice, we introduce asymmetric variations of the fit interval by shifting its endpoints by up to $50\%$ relative to the peak position. The resulting resonance parameters are shown in Fig.~\ref{fig:dos_fit_analysis}. We observe that the extracted resonance energy depends only very weakly on the fit interval, while the width shows a somewhat larger, but still moderate, variation.

\begin{figure*}[t]
    \centering
    \includegraphics[width=1\linewidth]{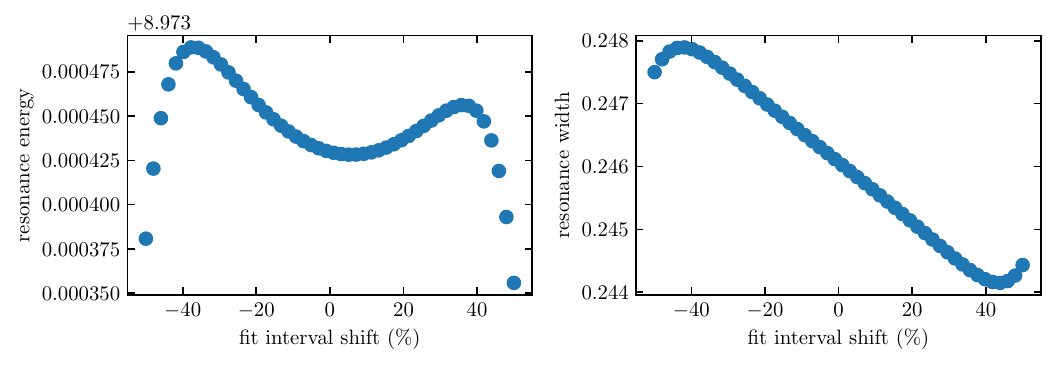}
    \caption{Resonance parameters from DOS fits of $N=8,9,10$ states for $G=20$ for shifted fit intervals.}
    \label{fig:dos_fit_analysis}
\end{figure*}

Overall, these results indicate that the DOS method is robust with respect to the choice of both averaging parameters and fit interval, and that the procedure adopted in the main text provides reliable and stable results.

\subsection{Fit to Quasi-Bound Probabilities}
We first analyze the dependence on the choice of the eigenstate by extracting resonance parameters for $N=5,10,15$. The resulting energies agree within three significant digits, while the widths show only very small deviations ($0.244$, $0.245$, $0.245$). This indicates weak dependence on $N$, and we therefore choose $N=10$ in the main analysis.

The fitting procedure itself is performed analogously to the DOS method, i.e., by fitting a Lorentzian profile in energy space using a symmetrically defined interval around the peak. The dependence on the fit interval is shown in Fig.~\ref{fig:qbp_fit_analysis}. As in the DOS case, the resonance energy exhibits weak dependence, while the width shows variation at the level of a few percents.

\begin{figure*}[t]
    \centering
    \includegraphics[width=1\linewidth]{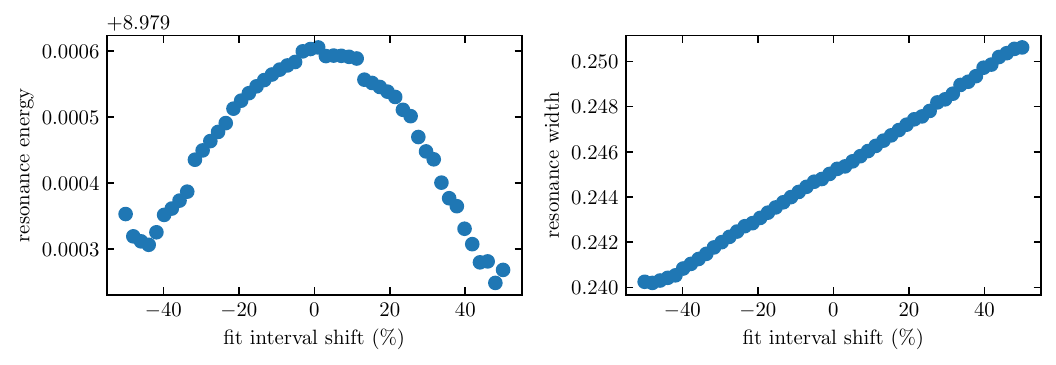}
    \caption{Resonance parameters from QBP fits of the $N=10$ state for $G=20$ for different shifted fit intervals.}
    \label{fig:qbp_fit_analysis}
\end{figure*}

In addition, the QBP method introduces a further parameter, namely the choice of the spatial region over which the quasi-bound probability is evaluated. In the main analysis, we integrate over the interior region $x\in[-a,0]$, corresponding to the region enclosed by the delta shell. To assess the sensitivity to this choice, we also extract resonance parameters by integrating over regions of the form $[-a,x_0]$, with $x_0=-0.4,-0.2,0,0.2,0.4,0.6$ (in units of $a$). The results are summarized in Table~\ref{tab:qbp_x0_analysis}. We find that the resonance energies remain stable within three significant digits for all choices of $x_0$. The widths, however, show a stronger variation when the integration region is restricted to a smaller interval. For integration regions that extend beyond the actual delta-shell region ($x_0 \geq 0$), the dependence of the widths becomes weak, indicating that the method is robust as long as the full interior region is included. Based on this observation, we conclude that the choice $x_0=0$ provides a natural and reliable definition of the interior region.

\begin{table}[t]
    \caption{Values of lowest resonance for $G=20$ extracted with the QBP method for different endpoints $x_0$ of the integration. Energies and widths are given in units of $\hbar^2/(2ma^2)$.}
    \label{tab:qbp_x0_analysis}

    \begin{ruledtabular}
    \begin{tabular}{c c c}
        $x_0/a$ & $E_\mathrm{r}$ & $\Gamma$ \\
        \hline
        $-0.4$ & $8.98$ & $0.408$ \\
        $-0.2$ & $8.98$ & $0.289$ \\
        $0.0$  & $8.98$ & $0.245$ \\
        $0.2$  & $8.98$ & $0.242$ \\
        $0.4$  & $8.98$ & $0.244$ \\
        $0.6$  & $8.98$ & $0.249$ \\
    \end{tabular}
    \end{ruledtabular}
\end{table}

\end{document}
